# Supplementary material for: Quadrupolar resonance spectroscopy of individual nuclei using a room-temperature quantum sensor
Source: arXiv:2405.14859 source file (2025-01-11)
Supplement: Supplementary file 1 [file supplement.pdf]

# Supporting Information: Quadrupolar resonance spectroscopy of individual nuclei using a room-temperature quantum sensor

S. Alex Breitweiser,<sup>1,2,\*</sup> Mathieu Ouellet,<sup>1,\*</sup> Tzu-Yung Huang,<sup>1,†</sup> Tim H. Taminiau,<sup>3,4</sup> and Lee C. Bassett<sup>1,‡</sup>

<sup>1</sup>*Quantum Engineering Laboratory, Department of Electrical and Systems Engineering,  
University of Pennsylvania, 200 S. 33rd St. Philadelphia, Pennsylvania, 19104, USA* §

<sup>2</sup>*Department of Physics and Astronomy, University of Pennsylvania,  
209 S. 33rd St. Philadelphia, Pennsylvania 19104, USA*

<sup>3</sup>*QuTech, Delft University of Technology, PO Box 5046, 2600, GA Delft, The Netherlands*

<sup>4</sup>*Kavli Institute of Nanoscience Delft, Delft University of Technology,  
PO Box 5046, 2600, GA Delft, The Netherlands*

(Dated: January 11, 2025)

## I. SAMPLE FABRICATION

The sample and setup are the same as those described in Refs. 1 and 2. In order to increase the photon collection efficiency, NV-A is located at the center of a 6- $\mu\text{m}$ -diameter solid immersion lens (SIL). To align and fabricate the SIL, we first spin-coated a 500 nm layer of PMMA A8 resist (MicroChem Nano PMMA) onto the diamond surface without baking the resist. After identifying a candidate NV in our confocal microscope, we used the 532 nm excitation laser to burn five holes into the PMMA: four marking the corners of an 8- $\mu\text{m}$  bounding box, and one centered over the NV center. Next, we sputtered a layer of AuPd onto the PMMA to mitigate charging during SIL fabrication. The sample was then loaded into a dual-beam scanning electron microscope and focused ion beam system (SEM/FIB, Strata D235, FEI), where the alignment marks were identified and the SIL was milled. After milling, a gallium-implanted layer remains on the diamond surface, which we removed by etching 80 nm of diamond using an Ar/Cl ICP/RIE process (Trion Phantom ICP, Pressure: 10 mT, ICP: 400 W, RIE: 300 W, Ar: 12 sccm, Cl<sub>2</sub>: 20 sccm) [3]. Finally, the sample was cleaned in Nanostrip (Cyantek) at 70° C for 20 minutes, followed by a soft O<sub>2</sub> plasma clean for 15 minutes (Anatech SCE-108 Barrel Asher, RF power = 30 W) to remove any graphite and to oxygen-terminate the surface. The microwave antenna was subsequently fabricated using standard optical lithography.

## II. ESR AND RAMSEY EXPERIMENTS

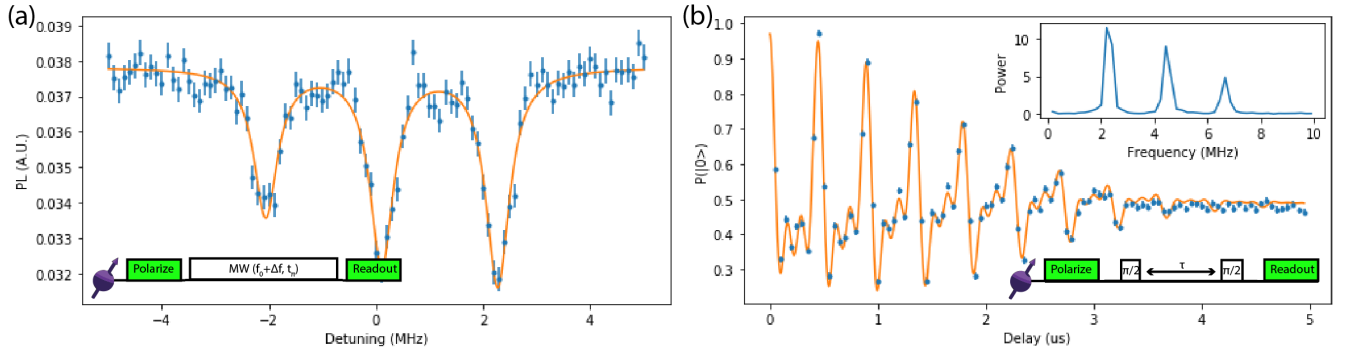

FIG. S1. (a) Pulsed ESR and (b) Ramsey data (blue points) from NV A taken with an on-axis field ( $B_Z > 0$ ). Fits (solid orange lines) are consistent with a model containing only the nitrogen-14 nuclear spin coupling, with no other strongly coupled spins detected.

\* These two authors contributed equally

† Present address: Nokia Bell Labs, 600 Mountain Avenue, Murray Hill, NJ 07974, USA

‡ lbassett@seas.upenn.edu

§ Present address: IBM Research, 1101 Kitchawan Rd Yorktown Heights, NY 10598, USA

With natural isotopic abundance, we expect around 1.1% of the carbon nuclei in the diamond lattice to be carbon-13. In bulk electronics grade samples, this means we expect a "typical" NV center to have a few carbon-13 nuclei coupled in the  $2\pi \times 10 - 100$  kHz range, as well as the NV's intrinsic nitrogen-14 nucleus with  $\approx 2\pi \times 2.17$  MHz coupling. It is possible to have more strongly coupled carbon-13 nuclei if one is located within the first few coordination shells around the NV center, which causes both the dipolar and contact couplings to increase. Two simple methods for measuring strong nuclear couplings are electron spin resonance (ESR) and Ramsey type experiments. These related experiments use either a weak, detuned microwave pulse or measure the rotation of a coherent electron superposition state to infer the energy levels of the electron spin. Since these are shifted by the coupling to nuclear spin, different frequencies will be observed. Both of these are limited in resolution by the coherence time of the electron, either under driving ( $T_2^{Rabi}$ ) or free decay ( $T_2^*$ ), which are expected to be similar.

Fig. S1 shows ESR and Ramsey data on NV A with an on axis magnetic field. In Fig. S1(a), ESR is taken with  $1 \mu s$  pulse widths at an amplitude which gives an approximate  $\pi$  rotation, leading to an  $\approx 1$  MHz resolution. While this does not saturate the coherence limit, this avoids broadening of the peaks due to slow spectral drift in the system. In Fig. S1, the phase of the final  $\frac{\pi}{2}$  pulse is swept at 5 MHz to aid in measuring the component oscillation frequencies of the beating signal. Data was taken past  $T_2^* \approx 2.4(1) \mu s$  and showed no revivals. Both of these datasets are consistent with a model including only the nitrogen-14 nuclear spin and no other strongly coupled nuclei ( $|A_Z| \gtrsim \frac{2\pi}{T_2^*} \approx 2\pi \times 300$  kHz, where  $|A_Z|$  is the strength of the on-axis component of the electro-nuclear hyperfine coupling). Datasets for the other NVs studied were similar, either showing no strong couplings or only a few couplings near the  $T_2^*$  limit for those with longer coherence times. None showed Carbon-13 couplings stronger than 200 kHz.

### III. DYNAMICAL DECOUPLING SPECTRUM

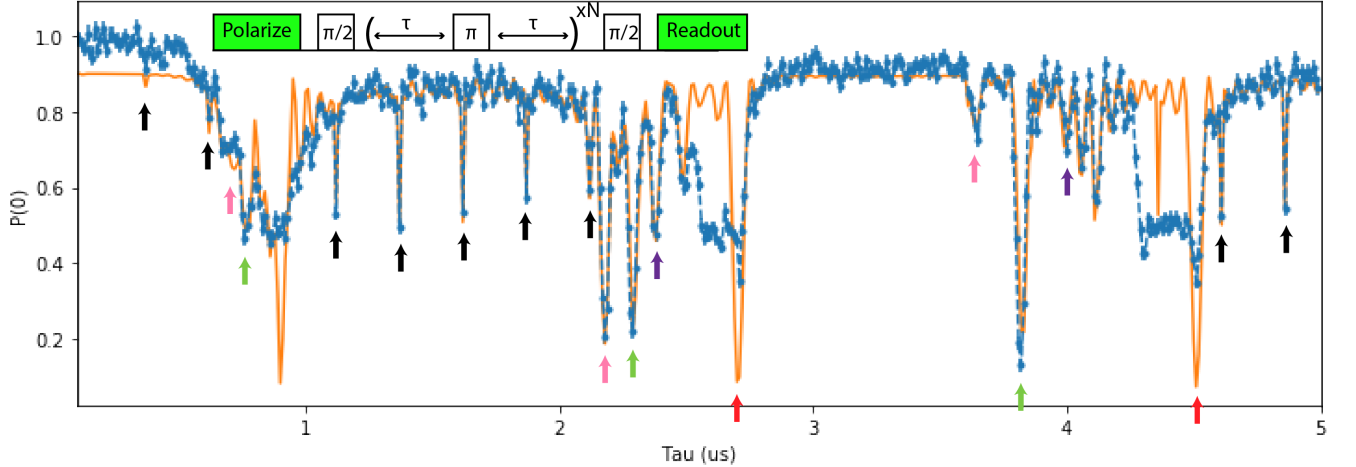

FIG. S2. Dynamical decoupling data (blue points w/ dashed line) taken on NV A with a purely on-axis field ( $B_X \approx 0$ ) shows resonances associated with multiple individual carbon-nuclei (colored arrows), as well as a resonance series associated with a higher energy spin (black arrows). Simulation (solid yellow line) shows this is consistent with an additional term in the nitrogen-14 nuclear quadrupolar Hamiltonian, as well as the known carbon-13 nuclei. Data is taken with  $N = 32$  pulses at a magnetic field of 264 Gauss aligned within  $\approx 1^\circ$  of the NV axis. (Inset) High-resolution data (markers) taken for various  $N$  around  $\tau = 1.372 \mu s$  fitted using our in-house simulator (best-fit simulation represented by dashed lines). Based on this we determine  $\alpha = 2\pi \times 2.43(2)$  kHz for the Nitrogen-14 nuclear spin.

Dynamical decoupling extends the coherence time of the electron spin with refocusing pulses. A single refocusing pulse is enough to extend the coherence time to several hundred  $\mu s$ , greatly increasing the resolution with which nuclear spin dynamics can be detected in spectroscopy. Furthermore, at higher pulse numbers and longer inter-pulse spacings, resonances from individual nuclei become sharper and separate spectrally, allowing resonances from weakly coupled nuclei to be observed. In the case of spin- $\frac{1}{2}$  nuclei such as  $^{13}C$ , the approximate location of individual nuclear spin resonances is given by

$$\tau_k = \frac{(2k-1)\pi}{2\omega_L + A_Z} \quad (1)$$

where  $\tau_k$  is the spacing between pulses at the  $k$ -th resonance,  $\omega_L$  is the nuclear Larmor frequency, and  $A_Z$  is the parallel component of the hyperfine coupling for that individual nuclei. Spectroscopy from sweeping  $\tau$  is then expected to reveal resonances arising from several more weakly coupled C-13 nuclei (with  $\frac{2\pi}{T_2} \gtrsim |A_Z| \gtrsim \frac{2\pi}{T_2} \approx 2\pi \times 10 \text{ kHz}$ ) for an NV in natural isotopic abundance diamond, such as those in the sample under study.

Indeed, we observe resonances associated with at least four C-13 nuclei within the dynamical decoupling spectroscopy data shown in Fig. S2, indicated by colored arrows. Additional data was taken at each resonance and fitted in simulation to obtain the hyperfine coupling for each carbon-13. In addition, broad resonances saturating to  $P(|0\rangle) = 0.5$  are caused by the electron spin entangling with a large number of nuclei near the carbon-13 Larmor frequency. Here, data is taken with a purely on-axis magnetic field ( $B_X \approx 0$ ), and therefore, resonances associated with the  $m_I = 0$  to  $m_I = \pm 1$  nitrogen nuclear spin transition are not expected to appear. However, the data also contain an unexpected, higher-frequency resonance series in addition to the expected carbon-13 resonances. The resonance series corresponds to a frequency of several MHz, and it is stable to the reorientation of the external DC magnetic field (up to at least  $\pm 3^\circ$ ). Additional data was taken around one of these resonances and fitted to obtain the  $\alpha$  and  $A$  parameters for the nitrogen-14 nuclear spin Hamiltonian in NV A as described in Fig. 2 of the main text. After fitting the four carbon-13 nuclear resonances and the nitrogen-14 nuclear parameters (including the  $P$  and  $A$  parameters) the simulations (yellow line) agree well with the dynamical decoupling spectra everywhere except near the carbon-13 Larmor frequency (which is expected as our exact simulations do not account for the nuclear spin bath).

Other NVs studied in this work showed similar carbon-13 resonances but did not display the high-frequency resonances associated with the nitrogen nuclear spin.

#### IV. FITTING ADDITIONAL HAMILTONIAN PARAMETERS FOR NITROGEN-14 NUCLEI

As described in the main text, data was taken for each NV with a slightly off-axis field ( $|B_X| > 0$ ), allowing  $m_I = 0$  to  $m_I = \pm 1$  nitrogen nuclear spin transitions to occur due to spin mixing. To fit the value of both the hyperfine and quadrupolar parameters of the Nitrogen nuclear spins in the NVs studied, the number of Dynamical Decoupling pulses was swept while looking at a narrow region around a high order resonances for each of the two transitions. The resonances were chosen to avoid features related to Carbon-13 nuclei coupled to each NV. The data for both resonances was simultaneously fitted to a simulation based on the Hamiltonian given in the main text for each NV, with the hyperfine and quadrupolar parameters allowed to vary. Additional variation parameters were added to account for the loss of coherence due to pulse imperfections and dephasing of the NV electron spin during the DD sequence. Data for each NV listed in the main text is shown in figure Fig. S3.

#### V. NUCLEAR SPIN INITIALIZATION AND TOMOGRAPHY SEQUENCES

Based on our fitted simulations, we find that  $N = 24$  pulses at a spacing of  $\tau = 1.372 \text{ us}$  gives an approximate  $\frac{\pi}{2}$  rotation between the  $|m_I = -1\rangle$  and  $|m_I = +1\rangle$  states of the Nitrogen-14 nuclear spin conditional on the state of the electron spin within the  $|m_S = 0\rangle / |m_S = -1\rangle$  manifold (see Fig1(b) of main text). Furthermore, simulations show that a high-fidelity unconditional  $Z$  rotation on the  $|m_I = \pm 1\rangle$  manifold of the Nitrogen-14 spin can be implemented using a single pulse on the  $|m_S = 0\rangle / |m_S = -1\rangle$  electron spin manifold, due to the small magnitude of the off-axis term in the nuclear quadrupolar Hamiltonian.

Using these two-qubit gates, we implement nuclear initialization and tomography sequences adapted from [5], as depicted in Fig. S4.

#### VI. INITIALIZED RAMSEY

As described in the main text, Ramsey data was taken after initializing the nitrogen nuclear spin using the above sequence to measure the population in each nuclear spin states. To ensure we are not observing a steady state polarization, the amount of green time used to re-initialize the electron spin is swept. Raw Ramsey data for each electron re-initialization length is shown in Fig. S5. Data for the steady state Ramsey is repeated from Fig. S1 As expected, the nuclear spin populations decay back to the steady state value due to off-axis hyperfine coupling in the excited electronic state, with a characteristic decay time of several  $\mu\text{s}$  (similar to other published work [6]).

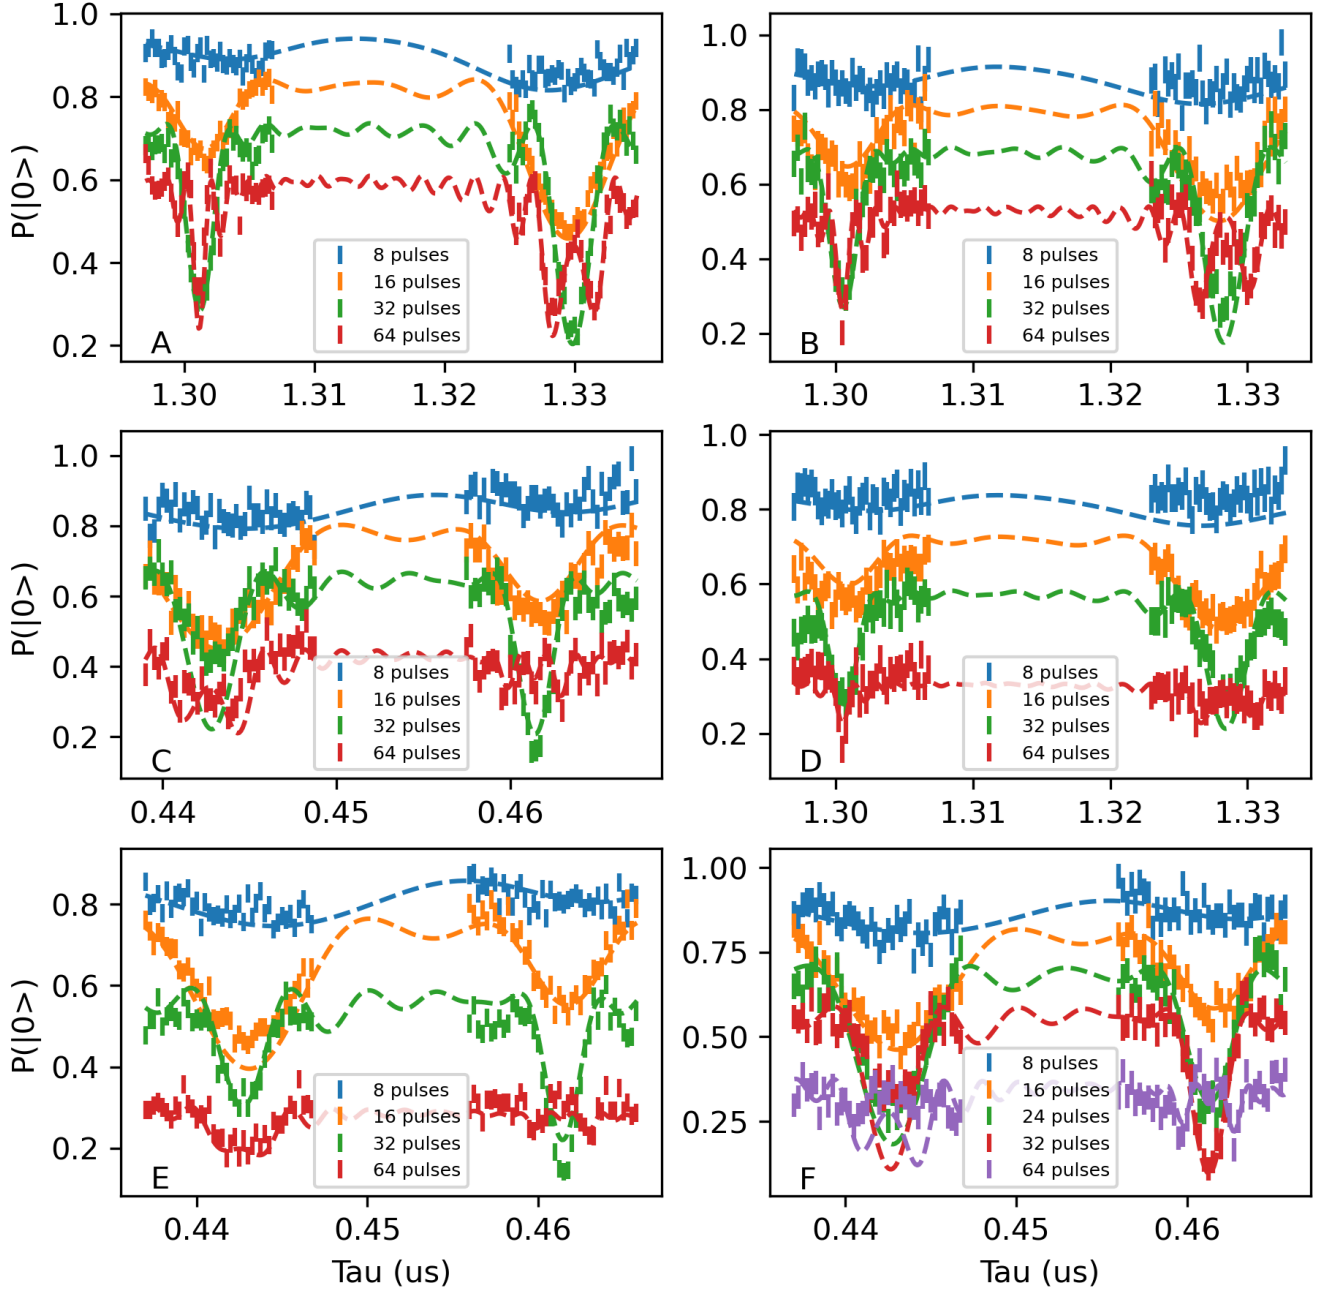

FIG. S3. Dynamical decoupling data for each NV studied taken with an off-axis field  $|B_X| > 0$ , showing resonances associated with  $|m_I = 0\rangle$  to  $|m_I = \pm 1\rangle$  transitions of the Nitrogen-14 nuclear spin as the number of dynamical decoupling pulses is swept. Pulse spacings below the hardware limit ( $\approx 1$  ns) are achieved using interpolated sequences [4]

## VII. FULL NITROGEN INITIALIZATION

### A. Simulations

Simulations throughout the manuscript were performed using exact simulation of the described Hamiltonians, along with the well-known Hamiltonian for the electronic spin of the negatively charged NV center at room temperature. Only spin degrees of freedom are considered, while optical and charge dynamics are assumed to be normalized away by readout calibrations which are interleaved with the experiments. Decoherence dynamics are modeled as a uniform decay of this signal, using the form described in Equation (8) of the main text. Hyperfine and quadrupolar parameters

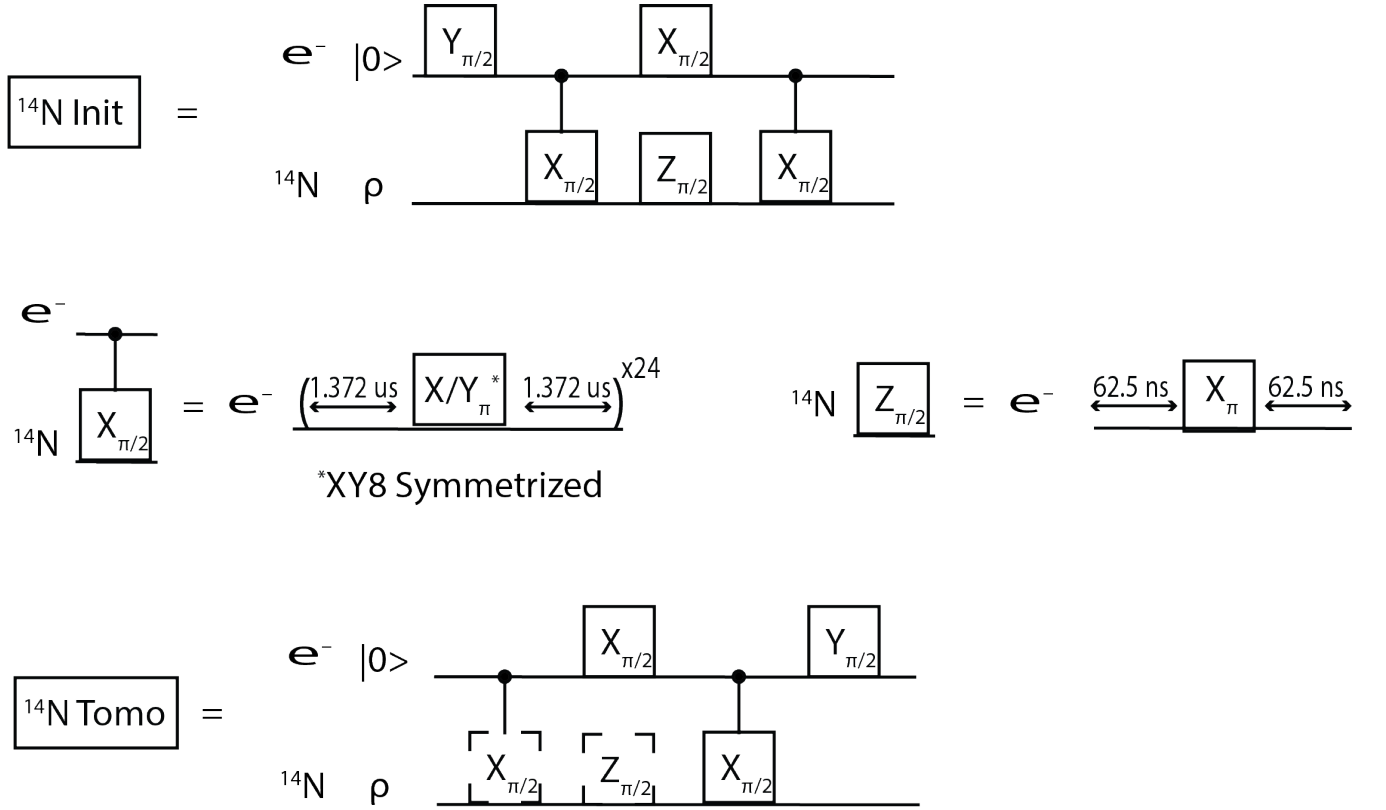

FIG. S4. Sequences used to initialize and read out the nuclear spin state using the electron spin. Dashed gates in the tomography sequence are included or removed depending on the desired nuclear measurement axis.

are extracted from data by allowing these parameters to vary in the simulations and fitting the simulation results to the data using general optimization methods.

In Figure 4, simulations are performed without (a) and with (b) Gaussian noise, which is representative of the dominant shot noise in our experiments. In Figure 4(a), the maximum contrast is obtained by sweeping the number of pulses and measuring the largest contrast obtained, where contrast is defined as the depth of the resonance peak divided by the total readout contrast (normalized to be 1). In Figure 4(b), simulations were performed and random noise was added in, using a noise amount characteristic of our experiments. For each value of  $\beta$ , the  $\alpha$  parameter in simulation was reduced until the uncertainty in the fit dropped below the actual signal.

### B. Resonant Lines for $\alpha$

The Hamiltonian of the system is given by:

$$\begin{aligned}
 H &= H_{ZE} + H_{ZN} + H_{hf} + H_{\text{quad}} \\
 H_{\text{quad}} &:= P(I_Z^2) + \alpha(I_+^2 + I_-^2) \\
 H_{hf} &:= A_Z S_Z I_Z + A_{\perp} S_Z I_X \\
 H_{ZE} &:= \Omega_E S_Z \\
 H_{ZN} &:= \Omega_N I_Z
 \end{aligned}$$

where  $H_{ZE}$  and  $H_{ZN}$  represent the Zeeman terms for the electronic and nitrogen spins, respectively,  $H_{\text{quad}}$  denotes the quadrupolar term, and  $H_{hf}$  refers to the hyperfine coupling between the two spins.

Under the assumption that the perpendicular hyperfine coupling is negligible, i.e.,  $A_{\perp} \approx 0$ , we can perform a unitary transformation  $U(t)$  to eliminate all the fast-rotating components from the system. The transformation is given by  $U(t) = e^{-i\Delta_E t S_z} \otimes e^{-i\Delta_N t I_z}$ . The transformation is described by  $U(t) = e^{-i\Delta_E t S_z} \otimes e^{-i\Delta_N t I_z}$ . Under this transformation, the terms  $H_{ZE}$ ,  $H_{ZN}$ , and  $H_{hf,Z}$  remain unchanged. Contrary to the isotropic components of the

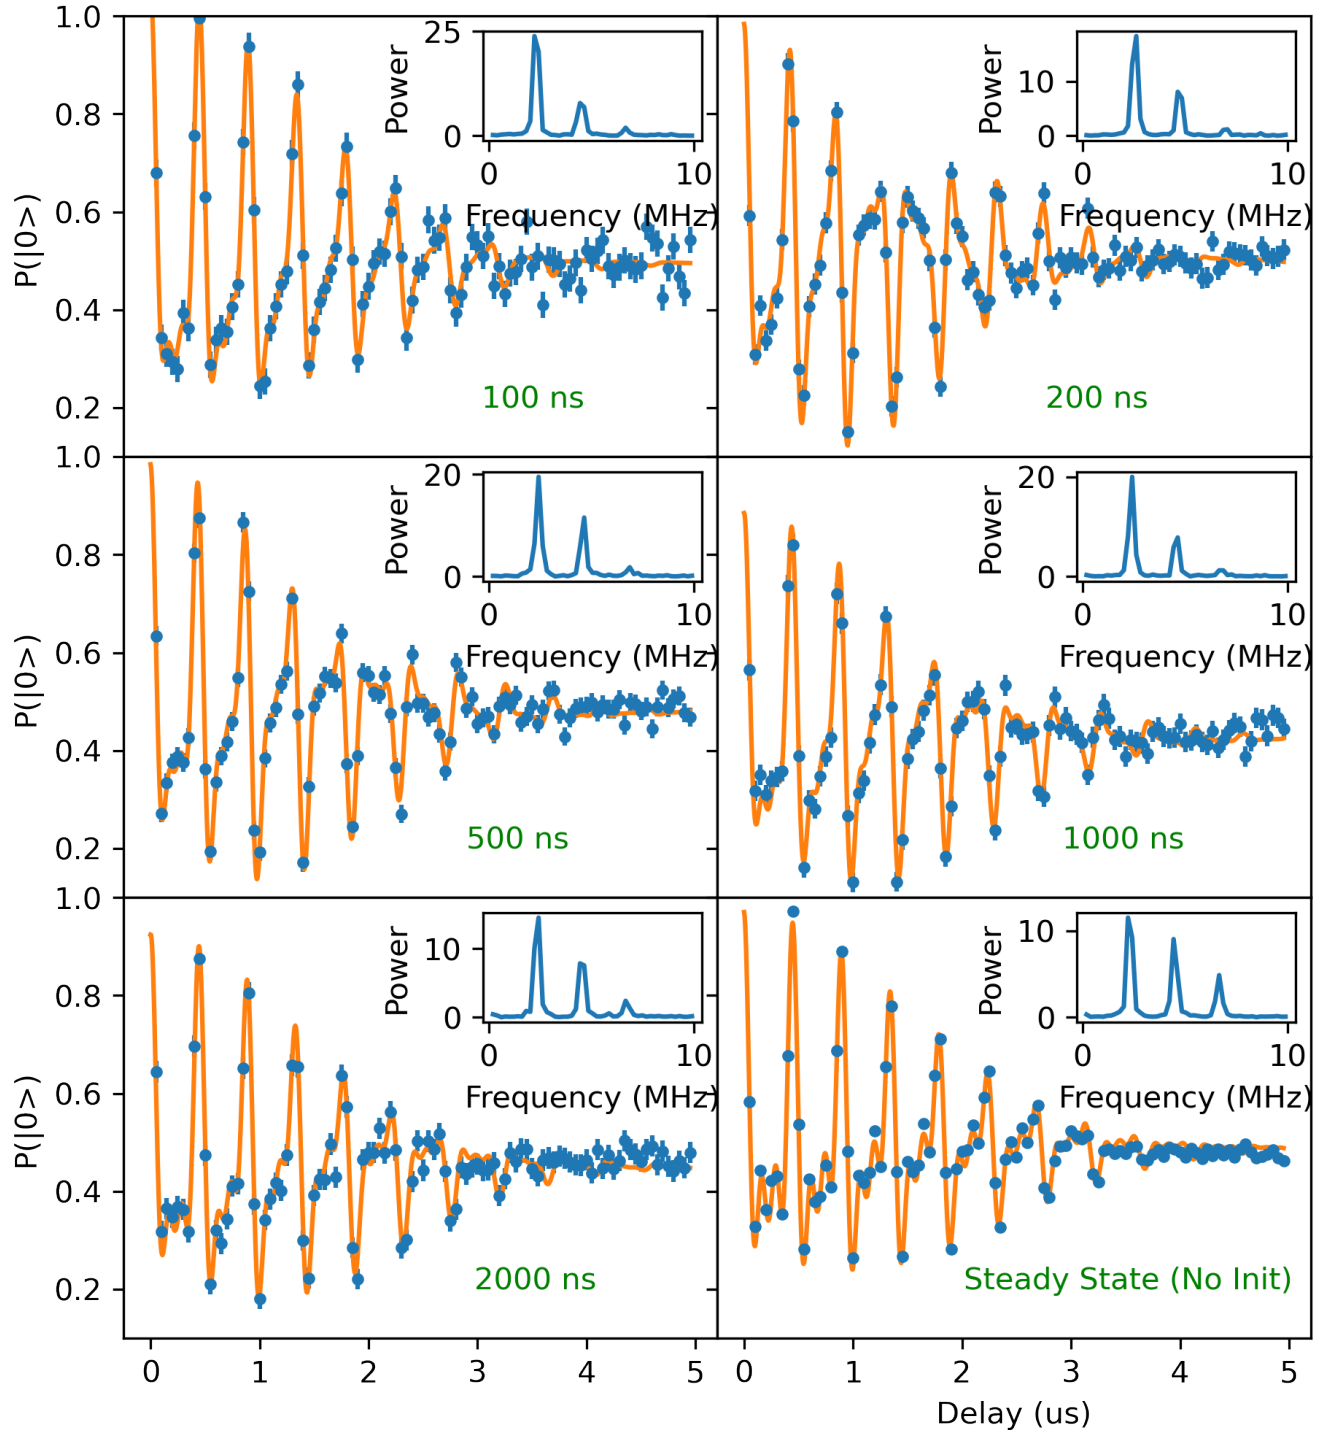

FIG. S5. Initialized Ramsey experiment for each of the electron re-initialization times, as depicted in Fig3(a) of the main text. Blue markers are data and yellow lines are oscillatory fits used to extract the occupation parameters of the Nitrogen-14 spin. (Insets) Power spectra for each of the Ramsey experiments - the polarization of the Nitrogen-14 spin is apparent from the unequal height of the frequency peaks.

Hamiltonian, the quadrupolar coupling does not commute with the other terms. As a result, it is essential to calculate its contribution to the Hamiltonian explicitly. Using the Baker–Campbell–Hausdorff formula, we get that

$$\begin{aligned} e^{i\lambda I_z} I_+^2 e^{-i\lambda I_z} &= e^{2i\lambda} I_+^2 \\ e^{i\lambda I_z} I_-^2 e^{-i\lambda I_z} &= e^{-2i\lambda} I_-^2 \end{aligned}$$

Thus, the Hamiltonian expressed in the rotating frame is given by:

$$H' = A_Z S_Z I_Z + P(I_Z^2) + \alpha(e^{2i\Delta_N} I_+^2 + e^{-2i\Delta_N} I_-^2)$$

where we set  $\Delta_E = \Omega_E$  and  $\Delta_N = \Omega_N$ . The term that is dependent on the electronic spin state is solely given by  $A_Z S_Z I_Z = A_Z [|1\rangle\langle 1| - |-1\rangle\langle -1|] \otimes I_Z$  which allows us to write the Hamiltonian as

$$H' = |-1\rangle\langle -1| \otimes H_{-1} + |0\rangle\langle 0| \otimes H_0 + |1\rangle\langle 1| \otimes H_1$$

where  $H_{-1} = -A_Z I_z + H_{ind}$ ,  $H_0 = H_{ind}$ , and  $H_1 = A_Z I_z + H_{ind}$ . We have consolidated the time-independent portion of the Hamiltonian into  $H_{ind}$ , which includes the quadrupolar term and is expressed as:

$$H_{ind} = P(I_Z^2) + \alpha(e^{2i\Delta_N} I_+^2 + e^{-2i\Delta_N} I_-^2)$$

The evolution operator  $V = \exp\{-iHt\}$  takes the same form

$$V = |-1\rangle\langle -1| \otimes V_{-1} + |0\rangle\langle 0| \otimes V_0 + |1\rangle\langle 1| \otimes V_1,$$

where  $V_i$  exclusively influences the nitrogen subspace with spin state  $i$  and can be formulated as a rotation around an axis  $\vec{n}_i$  of angle  $\phi_i$  such that  $V_i = \exp[-i\phi_i(\vec{I} \cdot \vec{n}_i)]$ . For a spin 1 system, the trace is computed as

$$\text{Tr} \left[ \exp \left[ -i\phi_i(\vec{I} \cdot \vec{n}) \right] \right] = 1 + 2 \cos \phi_i.$$

Our goal is to isolate  $\vec{n}_i \cdot \vec{n}_j$  to allow us to find the resonance conditions. To do so, we can use the fact that  $\text{Tr} \left[ \exp \left[ -i\phi(\vec{I} \cdot \vec{n}) \right] I_j \right] = -2i \sin(\phi) n_j$  to generate this expression

$$\vec{n}_{-1} \cdot \vec{n}_0 = 1 + \frac{1}{4} \sum_{j \in \{x, y, z\}} \frac{\text{Tr}[(V_{-1} - V_0)I_j] \text{Tr}[(V_{-1}I_j)]}{1 - \left( \frac{\text{Tr}[V_0] - 1}{2} \right)^2}$$

Under a  $\pi$ -pulse, using the  $|-1\rangle, |0\rangle$  as an example the electronic spin evolves as follows:  $|-1\rangle \rightarrow |0\rangle$ ,  $|+1\rangle \rightarrow |+1\rangle$ , and  $|0\rangle \rightarrow |-1\rangle$ , with the pulse sequence specified by:

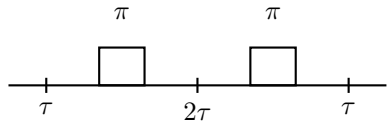

This results in the following evolution operators:

$$\begin{aligned} V_0 &= \exp[-i\tau H_{ind}] \exp[-2i\tau H_{+1}] \exp[-i\tau H_{ind}] \\ V_{-1} &= \exp[-4i\tau H_{-1}] \\ V_{+1} &= \exp[-i\tau H_{+1}] \exp[-2i\tau H_{ind}] \exp[-i\tau H_{+1}]. \end{aligned}$$

Our objective is to determine the difference in rotation between the  $+1$  and  $-1$  states, which can be computed as  $\vec{n}_{-1} \cdot \vec{n}_{+1}$  and the angle of rotation  $\phi$ . It is important to note that our aim is not to maximize the angle  $\phi$  but rather to find the condition that maximizes the difference in the evolution of the states  $|+1\rangle\langle +1|$  and  $|-1\rangle\langle -1|$ . Our goal is, therefore, to minimize the dot product between those two angles:

$$\tau_{res} = \arg \min_{\tau} \left( 1 + \frac{1}{4} \sum_{j \in \{x, y, z\}} \frac{\text{Tr}[(V_{+1} - V_{-1})I_j] \text{Tr}[(V_{+1}I_j)]}{1 - \left( \frac{\text{Tr}[V_{-1}] - 1}{2} \right)^2} \right)$$

Minimizing this equation is laborious, yet several small parameters are present in the Hamiltonian. The hyperfine coupling significantly outweighs the Zeeman term ( $\frac{\Omega_N}{A_Z} \approx 0.04$ ), allowing for a first-order expansion of the ratio. Similarly, for  $\frac{\alpha}{\Omega_N} \approx 0.03$ , retaining the term at first order is appropriate, while the term  $\frac{\alpha}{A_Z}$  can be safely omitted, as it is approximately 0.001.

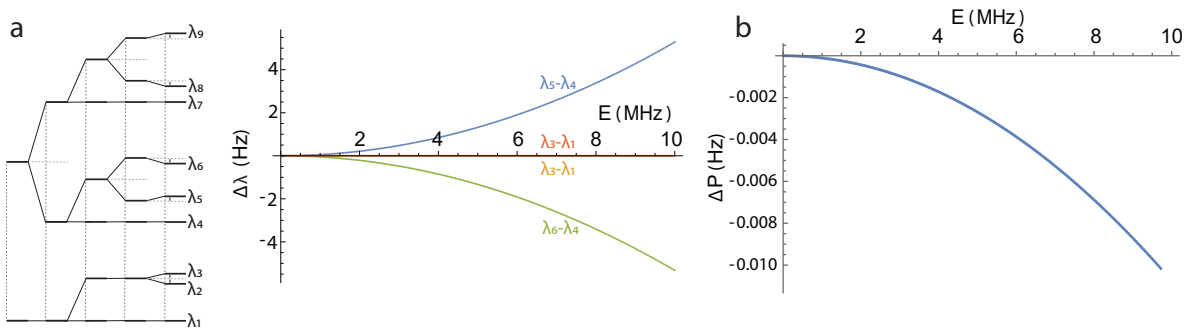

FIG. S6. Effect of a transverse electric or strain field (a) on the relative energy spacings in the  $m_s = 0$  and  $m_s = -1$  subspaces and (b) on the inferred nuclear quadrupolar splitting,  $P$ , as a function of the transverse zero-field splitting parameter,  $E$ .

### VIII. TRANSVERSE ELECTRIC OR STRAIN FIELDS

In this section, we consider potential contributions to the full electron-nuclear Hamiltonian and corresponding dynamics due to transverse electric fields or transverse strain fields. Transverse strain or electric fields break the NV center's symmetry [7], distorting the electron cloud and perturbing the zero-field electron-Hamiltonian parameters  $D$  and  $E$  (of which the latter should be strictly zero in the absence of such perturbation). In principle, these perturbations can combine with the hyperfine coupling to create second-order perturbations of the coupled electron-nuclear eigenstates and their corresponding energies. It is therefore important to confirm that the variations we observe in experiments cannot be explained by such perturbations.

Figure S6(a) shows the variation of the relative energy splittings within the  $m_s = 0$  and  $m_s = -1$  manifolds as a function of the electronic transverse perturbation,  $E_x$ . We observe that the transverse electronic term does indeed mix and perturb the coupled electron-nuclear states. However, for values of  $E$  on the scale of  $\sim 10$  MHz, as measured in our experiments, the corresponding perturbations are on the scale of a few hertz, which is several orders of magnitude smaller than the kHz-scale variations we observe in measurements of  $P$  and  $A_z$  (see Fig. 4 in the main text). Moreover, the perturbation tends to couple predominantly the  $m_I = 0$  states with  $m_I = \pm 1$ , such that the energy differences associated with  $\Delta m_I = \pm 1$  transitions evolve in opposite directions. In contrast, the longitudinal quadrupolar term  $P$  shifts both transitions in the same direction. Figure S6(b) illustrates this effect, where the change in effective  $P$  caused by transverse strain perturbations (effectively, the common-mode variation of the  $m_I = \pm 1$  levels compared to  $m_I = 0$ ) remains well below 1 Hz for relevant perturbation strengths. Higher-order electric-field perturbations (e.g., with an electronic Hamiltonian term proportional to  $S_Z S_X$ ) are typically neglected [8], and they result in an even smaller shift in the measured quadrupolar splitting.

Since the transverse-strain perturbations appear in the full Hamiltonian (Eq. 1 in the main text) as terms that couple  $m_I = 0$  states with  $m_I = \pm 1$  states, they are physically distinct from the nuclear quadrupolar asymmetry term,  $\alpha$ , which directly couples  $m_I = \pm 1$ . In this way, their effect would be similar (albeit smaller in magnitude) to the effect of an off-axis magnetic field, which also indirectly couples the states with  $\Delta m_I = 1$ . We have verified through simulations that such terms in the Hamiltonian cannot account for the regular series of dips that are associated with the direct  $\Delta m_I = 2$  transitions between states with  $m_I = \pm 1$ . This analysis further supports the interpretation of our model in capturing the observed frequency shifts in terms of variations in the nuclear quadrupolar Hamiltonian.

- 
- [1] David A Hopper, Richard R Grote, Annemarie L Exarhos, and Lee C Bassett. Near-infrared-assisted charge control and spin readout of the nitrogen-vacancy center in diamond. *Physical Review B*, 94(24):241201, 2016.
  - [2] David A. Hopper, Joseph D. Lauigan, Tzu-Yung Huang, and Lee C. Bassett. Real-time charge initialization of diamond nitrogen-vacancy centers for enhanced spin readout. *Phys. Rev. Appl.*, 13:024016, Feb 2020.
  - [3] Mohammad Jamali, Ilja Gerhardt, Mohammad Rezai, Karsten Frenner, Helmut Fedder, and Jörg Wrachtrup. Microscopic diamond solid-immersion-lenses fabricated around single defect centers by focused ion beam milling. *Review of Scientific Instruments*, 85(12), 2014.
  - [4] Ashok Ajoy, Yi-Xiang Liu, Kasturi Saha, Luca Marsegli, Jean-Christophe Jaskula, Ulf Bissbort, and Paola Cappellaro. Quantum interpolation for high-resolution sensing. *Proceedings of the National Academy of Sciences*, 114(9):2149–2153, 2017.
  - [5] T. H. Taminiau, J. Cramer, T. van der Sar, V. V. Dobrovitski, and R. Hanson. Universal control and error correction in

- multi-qubit spin registers in diamond. *Nature Nanotechnology*, 9(3):171–176, Mar 2014.
- [6] Tanmoy Chakraborty, Jingfu Zhang, and Dieter Suter. Polarizing the electronic and nuclear spin of the NV-center in diamond in arbitrary magnetic fields: analysis of the optical pumping process. *New Journal of Physics*, 19(7):073030, jul 2017.
  - [7] Florian Dolde, Helmut Fedder, Marcus W Doherty, Tobias Nöbauer, Florian Rempp, Gopalakrishnan Balasubramanian, Thomas Wolf, Friedemann Reinhard, Lloyd CL Hollenberg, Fedor Jelezko, et al. Electric-field sensing using single diamond spins. *Nature Physics*, 7(6):459–463, 2011.
  - [8] Eric Van Oort and Max Glasbeek. Electric-field-induced modulation of spin echoes of nv centers in diamond. *Chemical Physics Letters*, 168(6):529–532, 1990.
